# Supplementary material for: Robust On-Manifold Optimization for Uncooperative Space Relative Navigation with a Single Camera
Source: arXiv:2005.07110 source file (2020-05-14)
Supplement: Supplementary file 1 [file p_appendix.tex]

\section*{Appendix}

\subsection[Derivation of the Discrete-Time Process Noise Covariance Matrix]{Derivation of $\vect{\Gamma}(t,s)$}
\label{ap:pronoicov}

The discrete \gls{ekf} process noise covariance matrix is, by definition \cite{grewal2015kalman}, given by Eq. (\ref{eq:fil-gamma_mat_init}), where $\vect{\Phi}(t,s)$ is the error-state transition matrix, $\vect{G}(s)$ is the process noise input matrix, and $\vect{Q}(s)$ is the continuous-time process noise covariance (cf. Section \ref{sec:fil}). From Eq. (\ref{fil-eq:stm}), Eq. (\ref{eq:mp-liealgebra}), and Eq. (\ref{eq:mp-exp_map_so3}), $\vect{\Phi}(t,s)$ can be written in block matrix form as:
\begin{subequations}
\begin{equation}
    \begin{bmatrix} \vect{A} & \vect{E}\vect{A} & \vect{Z} & \vect{\Theta} \\
    \vect{0}_{3\times3} & \vect{A} & \vect{0}_{3\times3} & \vect{Z} \\
    \vect{0}_{3\times3} & \vect{0}_{3\times3} & \vect{I}_{3} & \vect{0}_{3\times3}\\
    \vect{0}_{3\times3} & \vect{0}_{3\times3} & \vect{0}_{3\times3} & \vect{I}_{3}\end{bmatrix},
\end{equation}
with
\begin{align}
    \vect{A} &= \vect{A}((t-s)\vect{\varpi}) = \exp_{\sothree}((t-s)\vect{\omega}),\\
    \vect{E} &= \vect{B}((t-s)\vect{\varpi}) = \left[ \vect{N}((t-s)\vect{\omega}) (t-s)\vect{\nu} \right]^\wedge,\\
    \vect{Z} &= \vect{Z}((t-s)\vect{\varpi}) = (t-s)\vect{M}((t-s)\vect{\omega}),\\
    \vect{\Theta} &= \vect{\Theta}((t-s)\vect{\varpi}) = (t-s)\vect{N}((t-s)\vect{\omega}),
\end{align}
\end{subequations}
and $\vect{\varpi}^\top = \icolsmall{\vect{\nu}^\top,\vect{\omega}^\top}$ taken to be evaluated at $\vecthat{\varpi}_{k-1}$. A diagonal structure is assumed for $\vect{Q}(s)$:
\begin{equation}
\begin{bmatrix}
\sigma_\nu^2 \vect{I}_3 & \vect{0}_{3\times3}\\
 \vect{0}_{3\times3} & \sigma_\omega^2 \vect{I}_3
\end{bmatrix},
\end{equation}
where $\sigma_\nu^2, \sigma_\omega^2$ are the linear and angular velocities covariances, respectively. Equation (\ref{eq:fil-gamma_mat_init}) can then be simplified:
\begin{equation}
    \vect{\Gamma}(t,s) =  \int\limits_{t_0}^t \begin{bmatrix}
    \sigma_\nu^2  \vect{Z} \vect{Z}^\top + \sigma_\omega^2  \vect{\Theta} \vect{\Theta}^\top & \sigma_\omega^2  \vect{\Theta} \vect{Z}^\top & \sigma_\nu^2  \vect{Z} & \sigma_\omega^2  \vect{\Theta}\\
    \sigma_\omega^2 \vect{Z} \vect{\Theta}^\top & \sigma_\omega^2 \vect{Z} \vect{Z}^\top & \vect{0}_{3\times3} & \sigma_\omega^2\vect{Z}\\
    \sigma_\nu^2 \vect{Z}^\top & \vect{0}_{3\times 3} & \sigma_\nu^2 \vect{I}_3 & \vect{0}_{3\times3}\\
    \sigma_\omega^2 \vect{\Theta}^\top & \sigma_\omega^2 \vect{Z}^\top  & \vect{0}_{3\times3} & \sigma_\omega^2 \vect{I}_3
    \end{bmatrix}  \urd s, \label{eq:ap-gamma_mat_rep}
\end{equation}
depending only on $\vect{Z}, \vect{\Theta}$, and on the covariances. The small angle approximation is applied to these two matrices in terms of $(t-s)\vect{\omega}$ to produce a simplified expression for them:
\begin{subequations}
\begin{align}
    \vect{Z} &\approx (t-s) \vect{I}_3 + \frac{(t-s)^2}{2}\vect{\omega}^\wedge,\\
    \vect{\Theta} &\approx \frac{(t-s)^2}{2}\vect{\nu}^\wedge  - \frac{(t-s)^3}{4\omega} \left(\vect{\omega}^\wedge \vect{\nu}^\wedge \vect{\omega}^{\wedge 2} + \vect{\omega}^{\wedge 2} \vect{\nu}^{\wedge 2} \vect{\omega}^\wedge\right)
\end{align}
\end{subequations}
with $\omega = \lVert \vect{\omega} \rVert$. This is a valid assumption for small inter-frame rotational motion, i.e. $(t-s)\omega \ll 1$. Replacing the quantities in Eq. (\ref{eq:ap-gamma_mat_rep}), integrating each entry is a lengthy task, but it only depends on the coefficient $(t-s)$. The obtained closed-form of the discrete-time process noise covariance is greatly simplified by dropping the terms with coefficient $(t-s)^n$ for $n>3$.
